# Supplementary material for: Exploring the Practicality of Generative Retrieval on Dynamic Corpora
Source: arXiv:2305.18952 source file (2024-10-05)
Supplement: Supplementary file 1 [file appendix_answer_recall_performance_deprecated.tex]

\begin{table*}[t]
    \centering
    %\tiny \hdashline[2pt/2pt]
    %\setlength\tabcolsep{1.5pt}
    \renewcommand{\arraystretch}{1.45}
    \resizebox{\textwidth}{!}{
\begin{tabular}{l|ccc|ccc|ccc|ccc}
\hline
 & \multicolumn{3}{c|}{answer recall at 5} & \multicolumn{3}{c|}{answer recall at 10} & \multicolumn{3}{c|}{answer recall at 50} & \multicolumn{3}{c}{answer recall at 100} \\ \hline
 & total & past & recent & total & past & recent & total & past & recent & total & past & recent \\ \hline
DE-past & 46.11\% & 36.55\% & 55.67\% & 55.09\% & 45.05\% & 65.13\% & 71.88\% & 64.25\% & 79.50\% & 78.13\% & 72.05\% & 84.20\% \\
DE & 59.23\% & 49.30\% & 69.17\% & 68.27\% & 58.90\% & 77.63\% & 82.96\% & 77.35\% & 88.57\% & 86.93\% & 82.85\% & 91.00\% \\
DE+2020 Q & 53.23\% & 37.60\% & 68.87\% & 60.83\% & 46.15\% & 75.50\% & 75.84\% & 66.05\% & 85.63\% & 81.16\% & 73.65\% & 88.67\% \\ \hline
GR-past & 55.85\% & 56.80\% & 54.90\% & 63.70\% & 64.50\% & 62.90\% & 77.60\% & 79.00\% & 76.20\% & 81.50\% & 82.80\% & 80.20\% \\
GR-full & 51.32\% & 50.90\% & 51.73\% & 58.53\% & 58.25\% & 58.80\% & 70.77\% & 70.60\% & 70.93\% & 74.40\% & 74.20\% & 74.60\% \\
GR-convent.LoRA & 52.52\% & 54.10\% & 50.93\% & 57.37\% & 56.30\% & 58.43\% & 65.92\% & 61.40\% & 70.43\% & 74.99\% & 76.25\% & 73.73\% \\
DynamicGR & 59.59\% & 59.20\% & 59.97\% & 67.41\% & 67.65\% & 67.17\% & 80.47\% & 81.30\% & 79.63\% & 84.09\% & 85.15\% & 83.03\% \\
DynamicGR+2020Q & 62.47\% & 60.00\% & 64.93\% & 70.25\% & 68.10\% & 72.40\% & 81.65\% & 80.30\% & 83.00\% & 85.02\% & 84.10\% & 85.93\% \\ \hline
\end{tabular}
}
    \caption{Full stats on the answer recall performance on dual encoder and generative retrieval variants. }
    \label{tabs:appendix_answer_recall_performance}
\end{table*}
