# Supplementary material for: Exploring the Practicality of Generative Retrieval on Dynamic Corpora
Source: arXiv:2305.18952 source file (2024-10-05)
Supplement: Supplementary file 2 [file appendix_hits_performance_deprecated.tex]

\begin{table*}[t]
    \centering
    %\tiny \hdashline[2pt/2pt]
    %\setlength\tabcolsep{1.5pt}
    \renewcommand{\arraystretch}{1.45}
    \resizebox{\textwidth}{!}{
\begin{tabular}{l|ccc|ccc|ccc|ccc}
\hline
 & \multicolumn{3}{c|}{hits at 5} & \multicolumn{3}{c|}{hits at 10} & \multicolumn{3}{c|}{hits at 50} & \multicolumn{3}{c}{hits at 100} \\ \hline
 & total & past & recent & total & past & recent & total & past & recent & total & past & recent \\ \hline
DE-past & 26.32\% & 18.20\% & 34.43\% & 32.17\% & 22.50\% & 41.83\% & 46.06\% & 34.25\% & 57.87\% & 52.13\% & 40.40\% & 63.87\% \\
DE & 39.81\% & 29.75\% & 49.87\% & 47.31\% & 35.85\% & 58.77\% & 62.63\% & 50.95\% & 74.30\% & 69.38\% & 58.35\% & 80.40\% \\
DE+2020 Q & 35.29\% & 20.55\% & 50.03\% & 41.14\% & 25.05\% & 57.23\% & 55.93\% & 39.10\% & 72.77\% & 61.04\% & 44.55\% & 77.53\% \\ \hline
GR-past & 33.15\% & 32.80\% & 33.50\% & 39.65\% & 38.90\% & 40.40\% & 54.15\% & 54.50\% & 53.80\% & 59.75\% & 60.60\% & 58.90\% \\
GR-full & 31.60\% & 31.50\% & 31.70\% & 37.19\% & 36.85\% & 37.53\% & 50.16\% & 49.55\% & 50.77\% & 56.88\% & 58.85\% & 54.90\% \\
GR-convent.Lora & 31.69\% & 32.00\% & 31.37\% & 37.63\% & 37.75\% & 37.50\% & 50.92\% & 51.80\% & 50.03\% & 55.24\% & 56.30\% & 54.17\% \\
DynamicGR & 38.08\% & 37.25\% & 38.90\% & 43.96\% & 43.15\% & 44.77\% & 58.49\% & 58.25\% & 58.73\% & 64.44\% & 64.40\% & 64.47\% \\
DynamicGR+2020Q & 41.01\% & 38.25\% & 43.77\% & 47.99\% & 45.30\% & 50.67\% & 62.90\% & 60.20\% & 65.60\% & 67.79\% & 65.00\% & 70.57\% \\ \hline
\end{tabular}
}
    \caption{Full stats on the hits performance on dual encoder and generative retrieval variants. }
    \label{tabs:appendix_hits_performance_deprecated}
\end{table*}
